# Supplementary material for: Effective Elastic Scaling of Deep Learning Workloads
Source: arXiv:2006.13878 source file (2020-06-24)
Supplement: Supplementary file 1 [file appendices.tex]

\section{Appendix}~\label{sec:discussion}

\subsection{Results: Comparison with Max- and Min-BS}
\label{appendix:compare_min_max}

Here we present our results mentioned in section~\ref{result:compare_min_max}

\subsection{Related Work : Commercial Offerings}
